# Supplementary material for: A Mountaineering Strategy to Excited States: Highly-Accurate Energies and Benchmarks for Bicyclic Systems
Source: arXiv:2109.13894 source file (2021-09-28)
Supplement: Supplementary file 1 [file M3-SI.pdf]

# A Mountaineering Strategy to Excited States: Highly-Accurate Energies and Benchmarks for Bicyclic Systems

# Supporting Information

Pierre-François Loos[†] and Denis Jacquemin[‡]

[†]*Laboratoire de Chimie et Physique Quantiques, Université de Toulouse, CNRS, UPS, France*

[‡]*Université de Nantes, CNRS, CEISAM UMR 6230, F-44000 Nantes, France*

E-mail:

# S1 Additional data and key MOs

LR-CCSD/*aug*-cc-pVTZ values for all considered transitions, together with the relevant MOs.

## S1.1 Azulene

Table S1: LR-CCSD/*aug*-cc-pVTZ ES data for azulene: symmetry, VTE (eV), oscillator strength, MO composition (absolute coefficient > 0.2) and nature of all considered ESs. The ordering of the states is the LR-CCSD one.

| | Sym. | $\Delta E$ | $f$ | MO | Nature |
|---|---|---|---|---|---|
| $S_1$ | $B_2$ | 2.278 | 0.005 | 34-38 (0.629) | Val ($\pi \rightarrow \pi^\star$) |
| $S_2$ | $A_1$ | 3.973 | 0.003 | 34-43 (-0.472); 33-38 (-0.447) | CT ($\pi \rightarrow \pi^\star$) |
| $S_3$ | $B_2$ | 4.780 | 0.052 | 33-43 (-0.550); 32-38 (-0.268) | CT ($\pi \rightarrow \pi^\star$) |
| $S_4$ | $A_2$ | 4.903 | | 34-35 (0.517); 34-37 (0.298) | Rydberg |
| $S_5$ | $A_1$ | 5.216 | 1.180 | 33-38 (0.469); 34-43 (-0.437) | Val ($\pi \rightarrow \pi^\star$) |
| $S_6$ | $B_1$ | 5.312 | 0.001 | 34-36 (-0.602); 34-50 (0.214) | Rydberg |
| $T_1$ | $B_2$ | 2.199 | | 34-38 (0.652) | Val ($\pi \rightarrow \pi^\star$) |
| $T_2$ | $A_1$ | 2.283 | | 34-43 (0.471); 33-38 (0.425) | Val ($\pi \rightarrow \pi^\star$) |
| $T_3$ | $A_1$ | 2.924 | | 33-38 (-0.485); 34-43 (0.426) | Val ($\pi \rightarrow \pi^\star$) |
| $T_4$ | $B_2$ | 4.180 | | 33-43 (-0.610) | Val ($\pi \rightarrow \pi^\star$) |

Figure S1: Selected HF/*aug*-cc-pVTZ molecular orbitals of azulene (contour: 0.04 au for valence MOs and 0.01 au for diffuse MOs).

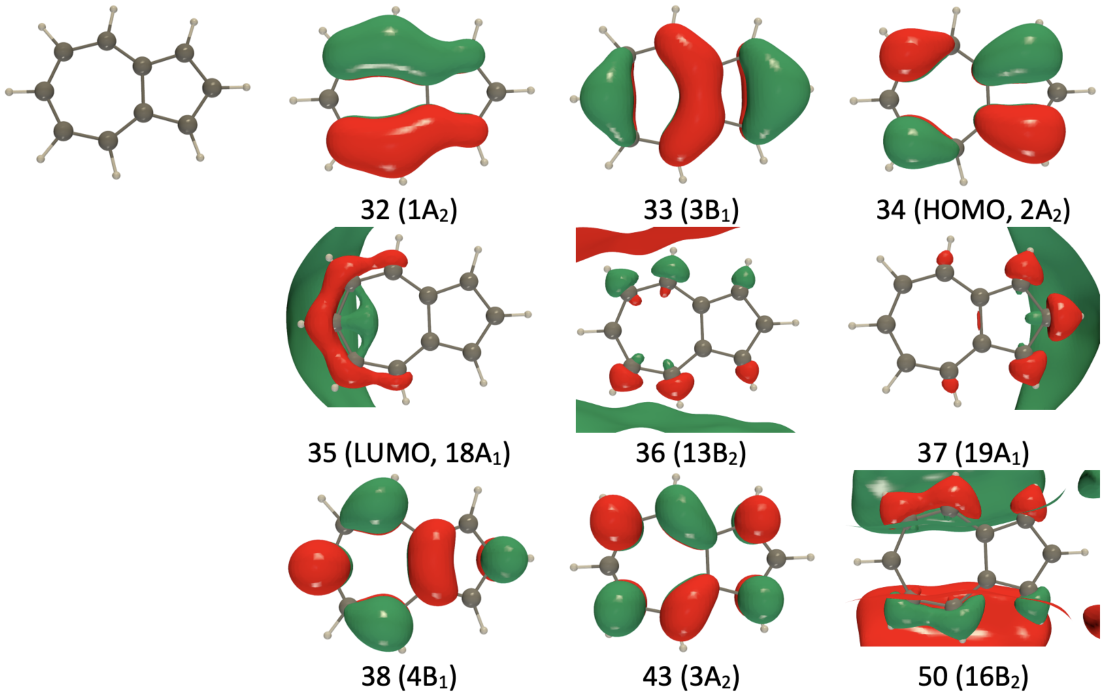

## S1.2 Benzoxadiazole

Table S2: LR-CCSD/*aug*-cc-pVTZ ES data for benzoxadiazole – see caption of Table S1 for more details.

| | Sym. | $\Delta E$ | $f$ | MO | Nature |
|---|---|---|---|---|---|
| $S_1$ | $B_2$ | 4.837 | 0.094 | 31-33 (0.655) | Val ($\pi \to \pi^\star$) |
| $S_2$ | $A_1$ | 5.221 | 0.076 | 30-33 (0.564) | Val ($\pi \to \pi^\star$) |
| $S_3$ | $A_2$ | 5.576 | | 28-33 (0.622) | Val ($n \to \pi^\star$) |
| $S_4$ | $B_1$ | 6.148 | 0.005 | 27-33 (0.618) | Val ($n/\sigma \to \pi^\star$) |
| $T_1$ | $B_2$ | 2.635 | | 31-33 (0.636) | Val ($\pi \to \pi^\star$) |
| $T_2$ | $A_1$ | 4.072 | | 30-33 (0.613) | Val ($\pi \to \pi^\star$) |

Figure S2: Selected HF/*aug*-cc-pVTZ molecular orbitals of benzoxadiazole (contour: 0.04 au).

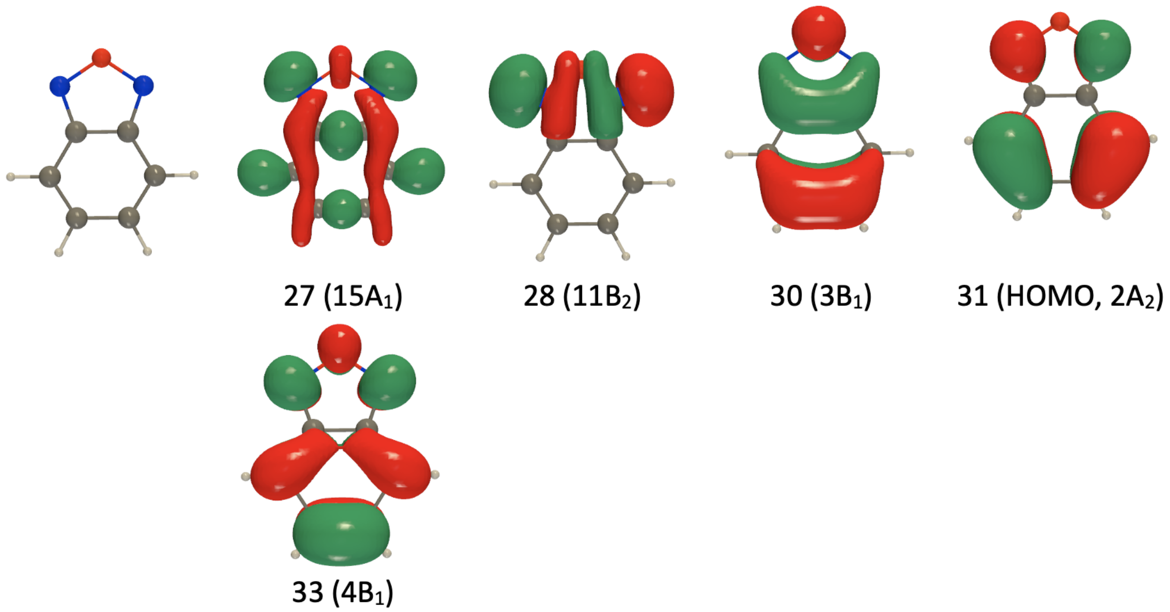

## S1.3 Benzothiadiazole

Table S3: LR-CCSD/*aug*-cc-pVTZ ES data for benzothiadiazole – see caption of Table S1 for more details.

| | Sym. | $\Delta E$ | $f$ | MO | Nature |
|---|---|---|---|---|---|
| $S_1$ | $A_1$ | 4.540 | 0.200 | 34-36 (0.604) | Val ($\pi \rightarrow \pi^\star$) |
| $S_2$ | $B_2$ | 4.559 | 0.053 | 35-36 (0.648) | CT ($\pi \rightarrow \pi^\star$) |
| $S_3$ | $A_2$ | 5.019 | | 32-36 (0.635) | Val ($n \rightarrow \pi^\star$) |
| $S_4$ | $B_1$ | 5.694 | 0.005 | 31-36 (0.625) | Val ($n/\sigma \rightarrow \pi^\star$) |
| $T_1$ | $B_2$ | 2.739 | | 35-36 (0.626) | Val ($\pi \rightarrow \pi^\star$) |
| $T_2$ | $A_1$ | 3.471 | | 34-36 (0.648) | Val ($\pi \rightarrow \pi^\star$) |

Figure S3: Selected HF/*aug*-cc-pVTZ molecular orbitals of benzothiadiazole (contour: 0.04 au).

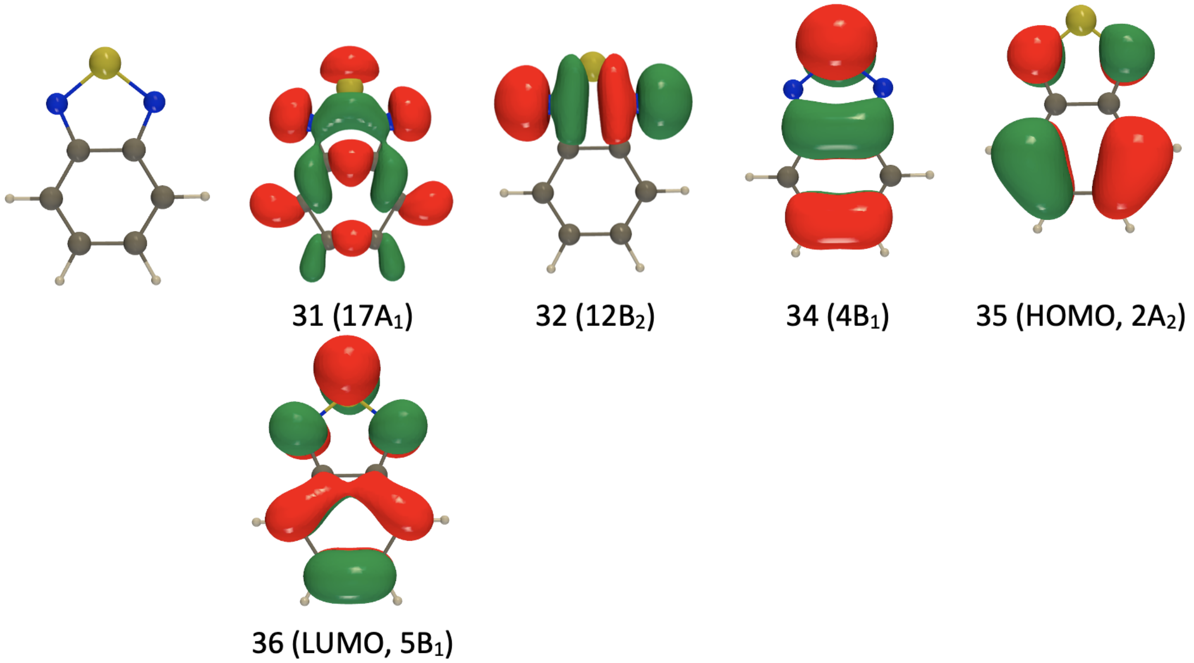

## S1.4 Diketopyrrolopyrrole

Table S4: LR-CCSD/*aug*-cc-pVTZ ES data for diketopyrrolopyrrole – see caption of Table S1 for more details.

| | Sym. | $\Delta E$ | $f$ | MO | Nature |
|---|---|---|---|---|---|
| $S_1$ | $B_u$ | 3.738 | 0.293 | 35-38 (0.625) | Val ($\pi \to \pi^\star$) |
| $S_2$ | $A_g$ | 4.209 | | 34-38 (0.625); 34-41 (-0.210) | Val ($\pi \to \pi^\star$) |
| $S_3$ | $A_u$ | 4.282 | 0.000 | 33-38 (0.592) | Val ($n \to \pi^\star$) |
| $S_4$ | $B_g$ | 4.745 | | 32-38 (-0.556); 33-55 (0.240) | Val ($n \to \pi^\star$) |
| $T_1$ | $B_u$ | 1.879 | | 35-38 (0.627) | Val ($\pi \to \pi^\star$) |
| $T_2$ | $A_g$ | 3.758 | | 34-38 (0.524); 32-55 (0.337) | Val ($\pi \to \pi^\star$) |
| $T_3$ | $A_u$ | 4.109 | | 33-38 (0.584) | Val ($n \to \pi^\star$) |
| $T_4$ | $B_g$ | 4.545 | | 32-38 (-0.545); 33-55 (0.258) | Val ($n \to \pi^\star$) |

Figure S4: Selected HF/*aug*-cc-pVTZ molecular orbitals of diketopyrrolopyrrole (contour: 0.04 au).

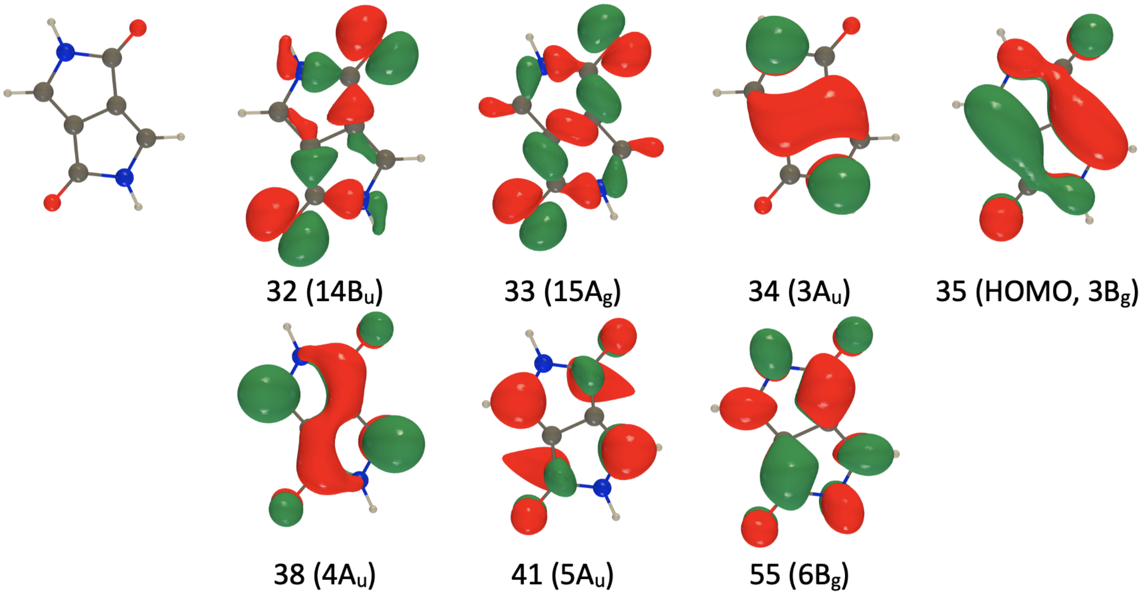

## S1.5 Furofruan

Table S5: LR-CCSD/*aug*-cc-pVTZ ES data for furofruan – see caption of Table S1 for more details.

| | Sym. | $\Delta E$ | $f$ | MO | Nature |
|---|---|---|---|---|---|
| $S_1$ | $A_u$ | 5.522 | 0.015 | 28-29 (0.564); 28-44 (-0.252) | Rydberg |
| $S_2$ | $B_u$ | 5.645 | 0.364 | 28-35 (0.506); 28-46 (-0.410) | Val ($\pi \rightarrow \pi^\star$) |
| $S_3$ | $B_g$ | 5.953 | | 28-30 (0.584); 28-40 (-0.224) | Rydberg |
| $S_4$ | $B_g$ | 6.109 | | 28-31 (0.544); 28-36 (-0.207) | Rydberg |
| $S_5$ | $A_u$ | 6.375 | 0.010 | 28-33 (-0.417); 28-29 (-0.264); 28-38 (-0.229) | Rydberg |
| $S_6$ | $A_g$ | 6.433 | | 28-53 (0.444); 28-41 (-0.408) | Val ($\pi \rightarrow \pi^\star$) |
| $S_7$ | $A_g$ | 6.511 | | 28-34 (0.657) | Rydberg |
| $T_1$ | $B_u$ | 3.516 | | 28-46 (0.501); 28-35 (-0.394) | Val ($\pi \rightarrow \pi^\star$) |
| $T_2$ | $A_g$ | 4.844 | | 28-53 (-0.418); 26-46 (0.294); 28-41 (0.272) | Val ($\pi \rightarrow \pi^\star$) |

Figure S5: Selected HF/*aug*-cc-pVTZ molecular orbitals of furofruan (contour: 0.04 au for valence and 0.01 au for diffuse MOs).

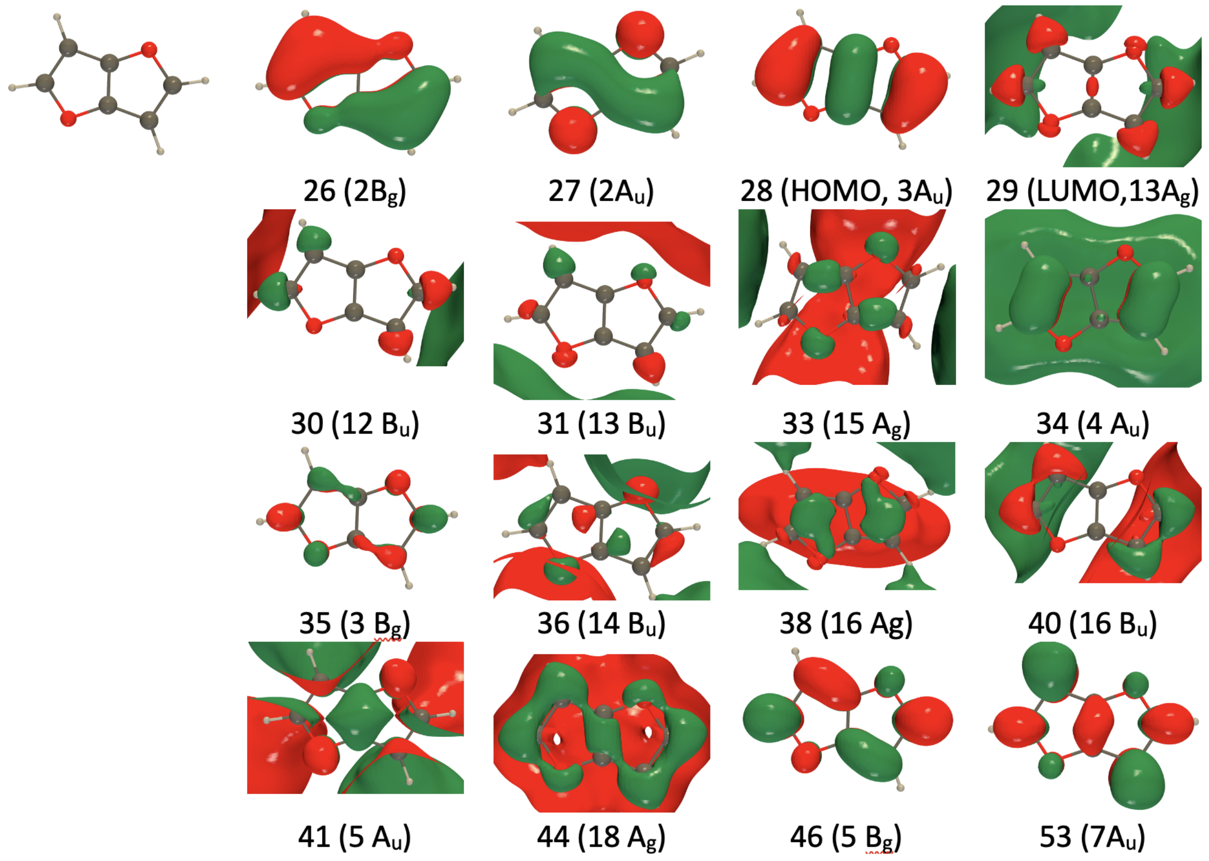

## S1.6 Phthalazine

Table S6: LR-CCSD/*aug*-cc-pVTZ ES data for phthalazine – see caption of Table S1 for more details.

| | Sym. | $\Delta E$ | $f$ | MO | Nature |
|---|---|---|---|---|---|
| $S_1$ | $A_2$ | 4.247 | | 32-40 (0.581) | CT ($n \to \pi^\star$) |
| $S_2$ | $B_1$ | 4.608 | 0.005 | 32-43 (0.602) | CT ($n \to \pi^\star$) |
| $S_3$ | $A_1$ | 4.642 | 0.004 | 34-43 (0.470); 33-40 (-0.420) | Val ($\pi \to \pi^\star$) |
| $S_4$ | $B_2$ | 5.368 | 0.053 | 34-40 (-0.605); 33-43 (-0.219) | Val ($\pi \to \pi^\star$) |
| $S_5$ | $B_1$ | 5.908 | 0.003 | 30-40 (-0.574) | CT ($n \to \pi^\star$) |
| $S_6$ | $A_2$ | 6.224 | | 30-43 (0.601) | CT ($n \to \pi^\star$) |
| $S_7$ | $A_1$ | 6.422 | 0.002 | 31-43 (-0.461); 33-62 (0.263) | Val ($\pi \to \pi^\star$) |
| $S_8$ | $A_2$ | 6.517 | | 34-35 (-0.539); 34-37 (-0.216) | Rydberg |
| $S_9$ | $A_2$ | 6.541 | | 32-42 (0.407); 32-62 (0.347); 32-40 (0.209) | Mixed |
| $S_{10}$ | $B_2$ | 6.546 | 0.034 | 32-37 (-0.395); 32-35 (-0.332) | Rydberg |
| $S_{11}$ | $A_1$ | 6.650 | 1.286 | 33-40 (0.476); 34-43 (0.425) | Val ($\pi \to \pi^\star$) |
| $S_{12}$ | $B_2$ | 6.660 | 0.100 | 33-43 (0.467); 34-42 (0.245); 34-62 (0.220) | Val ($\pi \to \pi^\star$) |
| $T_1$ | $B_2$ | 3.319 | | 34-40 (-0.575); 33-43 (-0.213) | Val ($\pi \to \pi^\star$) |
| $T_2$ | $A_2$ | 3.891 | | 32-40 (0.559) | CT ($n \to \pi^\star$) |
| $T_3$ | $B_1$ | 3.899 | | 32-43 (-0.564) | CT ($n \to \pi^\star$) |
| $T_4$ | $A_1$ | 4.315 | | 34-43 (0.547); 33-40 (0.302) | Val ($\pi \to \pi^\star$) |

Figure S6: Selected HF/*aug*-cc-pVTZ molecular orbitals of phthalazine (contour: 0.04 au for valence MOs, 0.01 au for diffuse MOs, and 0.02 au for MO n$^o$42).

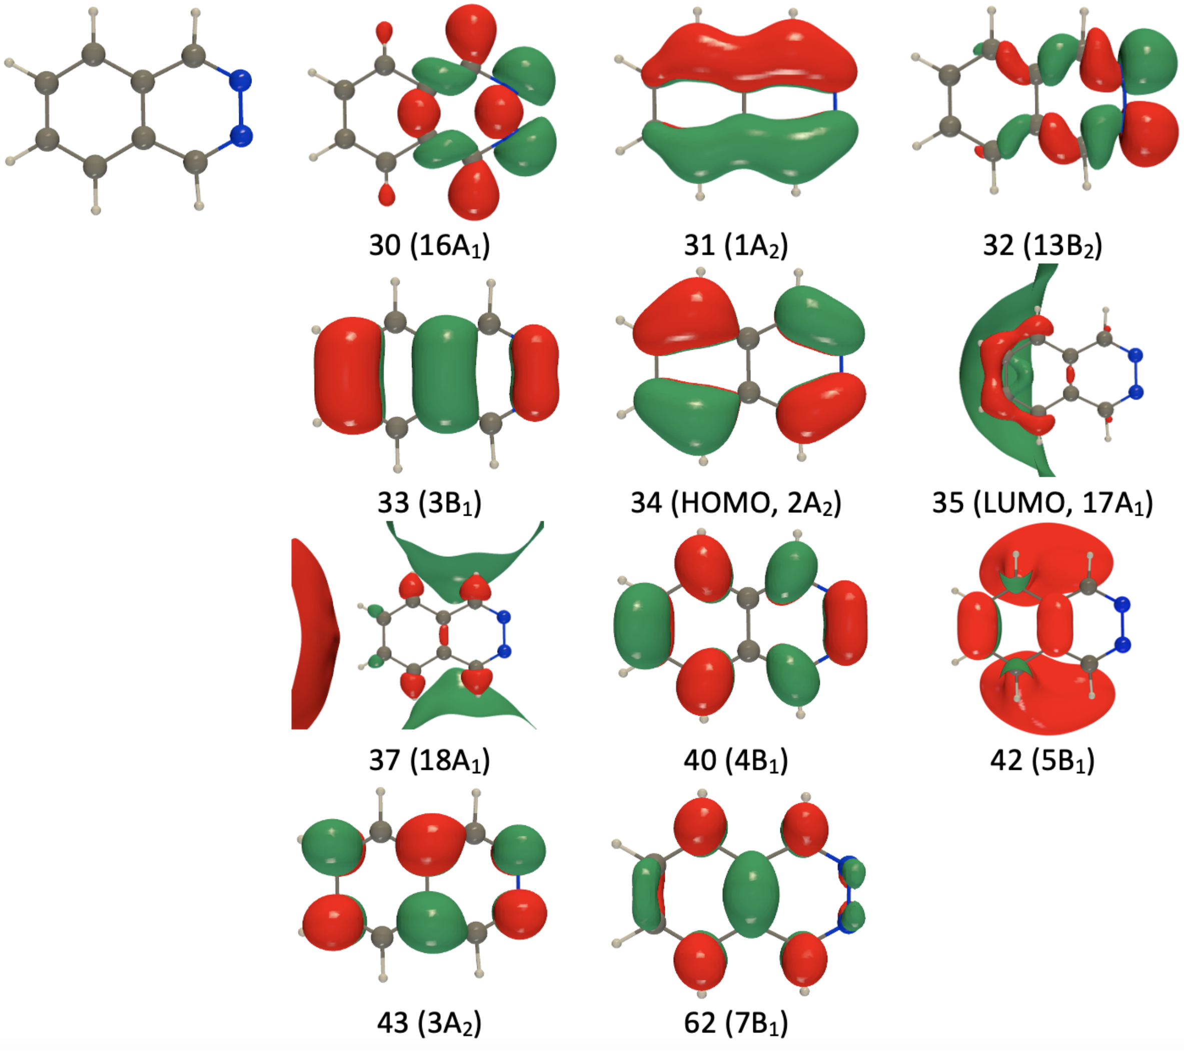

## S1.7 Pyrrolopyrrole

Table S7: LR-CCSD/*aug*-cc-pVTZ ES data for pyrrolopyrrole – see caption of Table S1 for more details.

| | Sym. | $\Delta E$ | $f$ | MO | Nature |
|---|---|---|---|---|---|
| $S_1$ | $A_u$ | 4.653 | 0.010 | 28-29 (-0.604); 28-44 (0.241) | Rydberg |
| $S_2$ | $B_g$ | 4.842 | | 28-30 (0.579); 28-39 (-0.224) | Rydberg |
| $S_3$ | $A_u$ | 5.191 | 0.000 | 27-29 (0.586); 27-44 (-0.250) | Rydberg |
| $S_4$ | $B_g$ | 5.201 | | 28-31 (0.604); 28-41 (-0.201) | Rydberg |
| $T_1$ | $B_u$ | 3.782 | | 28-51 (0.497); 28-53 (-0.319); 28-36 (-0.247) | Val ($\pi \rightarrow \pi^\star$) |
| $T_2$ | $A_u$ | 4.596 | | 28-29 (0.598); 28-44 (-0.244) | Rydberg |
| $T_3$ | $B_g$ | 4.823 | | 28-30 (-0.578); 28-39 (0.234) | Rydberg |

Figure S7: Selected HF/*aug*-cc-pVTZ molecular orbitals of pyrrolopyrrole (contour: 0.04 au for valence MOs, 0.01 au for diffuse MOs, and 0.02 au for MO n$^o$36).

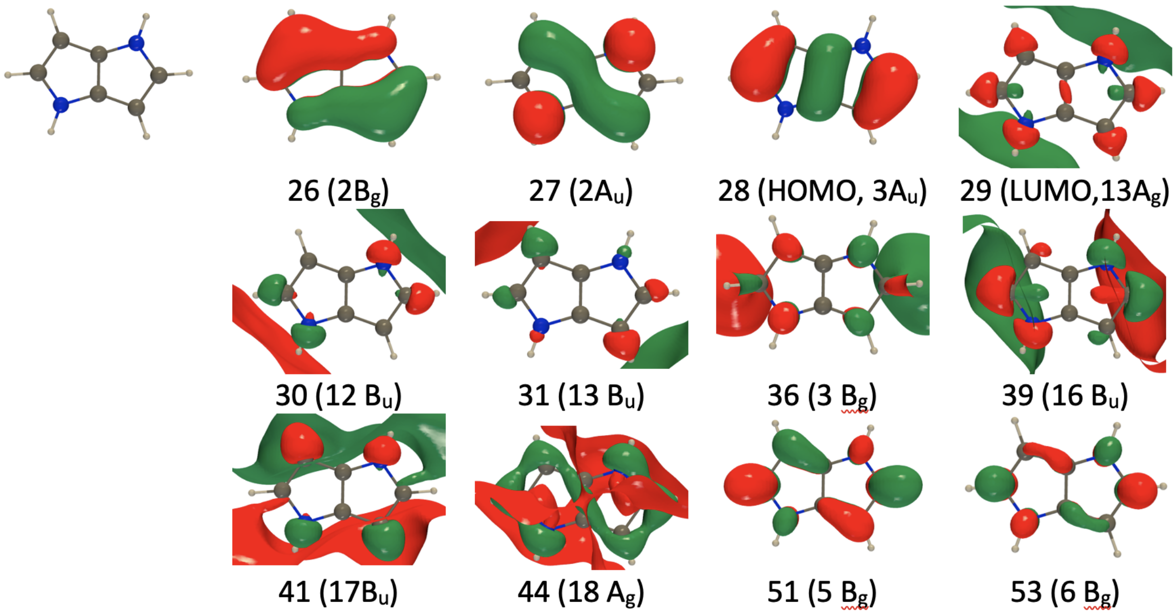

## S1.8 Quinoxaline

Table S8: LR-CCSD/*aug*-cc-pVTZ ES data for quinoxaline – see caption of Table S1 for more details.

| | Sym. | $\Delta E$ | $f$ | MO | Nature |
|---|---|---|---|---|---|
| $S_1$ | $B_1$ | 4.016 | 0.004 | 32-39 (-0.613) | Val ($n \rightarrow \pi^\star$) |
| $S_2$ | $A_1$ | 4.428 | 0.072 | 33-39 (0.534); 34-44 (0.235); 34-47 (-0.223) | Val ($\pi \rightarrow \pi^\star$) |
| $S_3$ | $B_2$ | 4.906 | 0.031 | 34-39 (-0.622) | CT ($\pi \rightarrow \pi^\star$) |
| $S_4$ | $A_2$ | 5.383 | | 32-44 (0.420); 32-47 (-0.336); 29-39 (-0.276) | Val ($n \rightarrow \pi^\star$) |
| $S_5$ | $A_2$ | 5.811 | | 29-39 (-0.530); 32-44 (-0.220) | Val ($n \rightarrow \pi^\star$) |
| $S_6$ | $A_1$ | 5.912 | 0.388 | 34-44 (-0.309); 33-50 (0.300); 34-47 (0.257) | Val ($\pi \rightarrow \pi^\star$) |
| $S_7$ | $B_2$ | 6.487 | 0.034 | 33-44 (0.391); 33-47 (-0.329); 34-50 (0.297) | Val ($\pi \rightarrow \pi^\star$) |
| $S_8$ | $A_2$ | 6.496 | | 34-35 (-0.501); 34-36 (-0.293); 34-55 (0.207) | Rydberg |
| $S_9$ | $B_1$ | 6.726 | 0.006 | 32-50 (0.477); 32-64 (-0.350) | CT ($\pi \rightarrow \pi^\star$) |
| $S_{10}$ | $B_1$ | 6.813 | 0.020 | 33-35 (-0.552); 33-55 (0.217) | Rydberg |
| $T_1$ | $B_2$ | 3.173 | | 34-39 (-0.567) | Val ($\pi \rightarrow \pi^\star$) |
| $T_2$ | $B_1$ | 3.494 | | 32-39 (0.596) | Val ($n \rightarrow \pi^\star$) |
| $T_3$ | $A_1$ | 3.923 | | 33-39 (0.609) | Val ($\pi \rightarrow \pi^\star$) |

Figure S8: Selected HF/*aug*-cc-pVTZ molecular orbitals of auinoxaline (contour: 0.04 au for valence MOs, and 0.01 au for diffuse MOs).

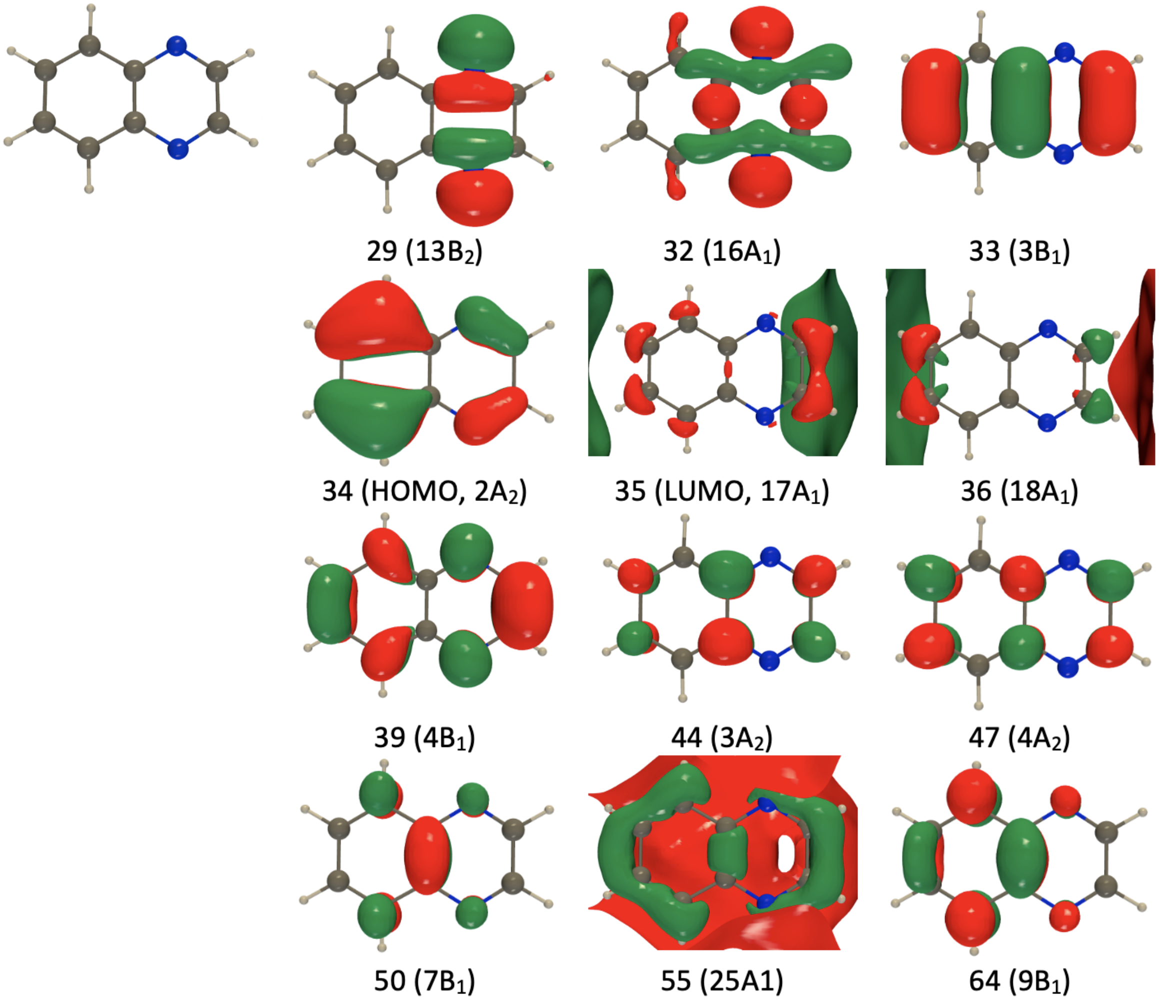

## S1.9 Tetrathiafulvalene

Table S9: LR-CCSD/*aug*-cc-pVTZ ES data for tetrathiafulvalene – see caption of Table S1 for more details.

| | Sym. | $\Delta E$ | $f$ | MO | Nature |
|---|---|---|---|---|---|
| $S_1$ | $B_{3u}$ | 3.019 | 0.001 | 52-66 (0.550); 52-60 (-0.233) | Val ($\pi \rightarrow \sigma^\star$) |
| $S_2$ | $B_{2u}$ | 4.088 | 0.053 | 52-63 (-0.575); 52-84 (0.236); 52-68 (0.212) | Val ($\pi \rightarrow \pi^\star$) |
| $S_3$ | $B_{1g}$ | 4.194 | | 52-69 (-0.374); 52-90 (0.326); 52-55 (0.265) | Val ($\pi \rightarrow \sigma^\star$) |
| $S_4$ | $B_{3u}$ | 4.224 | 0.024 | 52-54 (0.507); 52-60 (0.279); 52-57 (0.235) | Rydberg |
| $S_5$ | $B_{2g}$ | 4.238 | | 52-85 (-0.359); 52-53 (-0.296); 52-59 (0.288) | Val ($\pi \rightarrow \sigma^\star$) |
| $S_6$ | $B_{3g}$ | 4.584 | | 52-67 (-0.463);52-77 (0.422) | Val ($\pi \rightarrow \pi^\star$) |
| $S_7$ | $B_{1u}$ | 4.681 | 0.372 | 52-72 (-0.518); 52-61 (-0.360) | Val ($\pi \rightarrow \pi^\star$) |
| $S_8$ | $B_{2g}$ | 4.683 | | 52-53 (-0.523); 52-85 (0.234) | Rydberg |
| $T_1$ | $B_{3u}$ | 2.840 | | 52-66 (0.552); 52-60 (-0.227) | Val ($\pi \rightarrow \sigma^\star$) |
| $T_2$ | $B_{1u}$ | 2.961 | | 52-72 (-0.538); 52-61 (-0.258); 52-83 (0.245) | Val ($\pi \rightarrow \pi^\star$) |
| $T_3$ | $B_{2u}$ | 3.211 | | 52-63 (0.502); 52-84 (-0.240); 51-77 (-0.220) | Val ($\pi \rightarrow \pi^\star$) |
| $T_4$ | $B_{3g}$ | 3.438 | | 52-77 (-0.375); 52-67 (0.353); 51-63 (0.312) | Val ($\pi \rightarrow \pi^\star$) |
| $T_5$ | $B_{1g}$ | 3.972 | | 52-69 (0.356); 52-90 (-0.338); 52-80 (0.262) | Val ($\pi \rightarrow \sigma^\star$) |
| $T_6$ | $B_{2g}$ | 4.056 | | 52-85 (-0.394); 52-59 (0.279); 51-66 (-0.260) | Val ($\pi \rightarrow \sigma^\star$) |

Figure S9: Selected HF/*aug*-cc-pVTZ molecular orbitals of tetrathiafulvalene (contour: 0.04 au for valence MOs, 0.01 au for diffuse MOs, and 0.02 au for MO n$^o$61, 68, and 85).

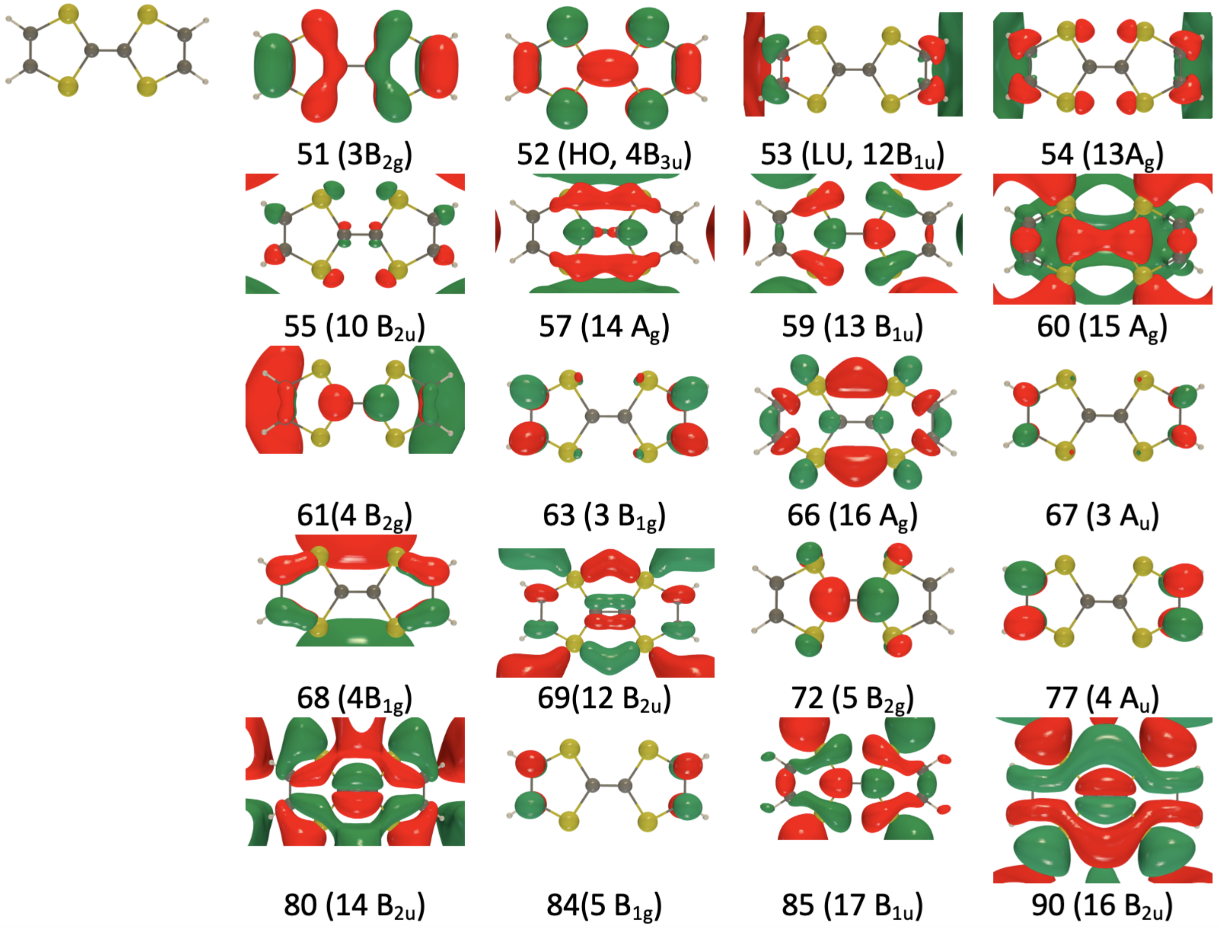

## S1.10 Thienothiophene

Table S10: LR-CCSD/*aug*-cc-pVTZ ES data for thienothiophene – see caption of Table S1 for more details.

| | Sym. | $\Delta E$ | $f$ | MO | Nature |
|---|---|---|---|---|---|
| $S_1$ | $B_u$ | 5.165 | 0.159 | 35-44 (-0.530); 36-44 (0.249) | Val ($\pi \rightarrow \pi^\star$) |
| $S_2$ | $B_u$ | 5.395 | 0.188 | 36-44 (0.549); 35-44 (0.285) | Val ($\pi \rightarrow \pi^\star$) |
| $S_3$ | $B_g$ | 5.600 | | 36-37 (0.299); 36-48 (-0.211) | Rydberg |
| $S_4$ | $A_u$ | 5.647 | 0.002 | 36-38 (-0.488); 36-50 (0.205); 36-40 (0.203) | Rydberg |
| $T_1$ | $B_u$ | 3.391 | | 36-44 (-0.590); 36-49 (-0.201) | Val ($\pi \rightarrow \pi^\star$) |
| $T_2$ | $B_u$ | 4.312 | | 35-44 (-0.601) | Val ($\pi \rightarrow \pi^\star$) |
| $T_3$ | $A_g$ | 4.555 | | 36-64 (-0.390); 34-44 (-0.326); 36-51 (-0.259) | Val ($\pi \rightarrow \pi^\star$) |

Figure S10: Selected HF/*aug*-cc-pVTZ molecular orbitals of thienothiophene (contour: 0.04 au for valence MOs, and 0.01 au for diffuse MOs).

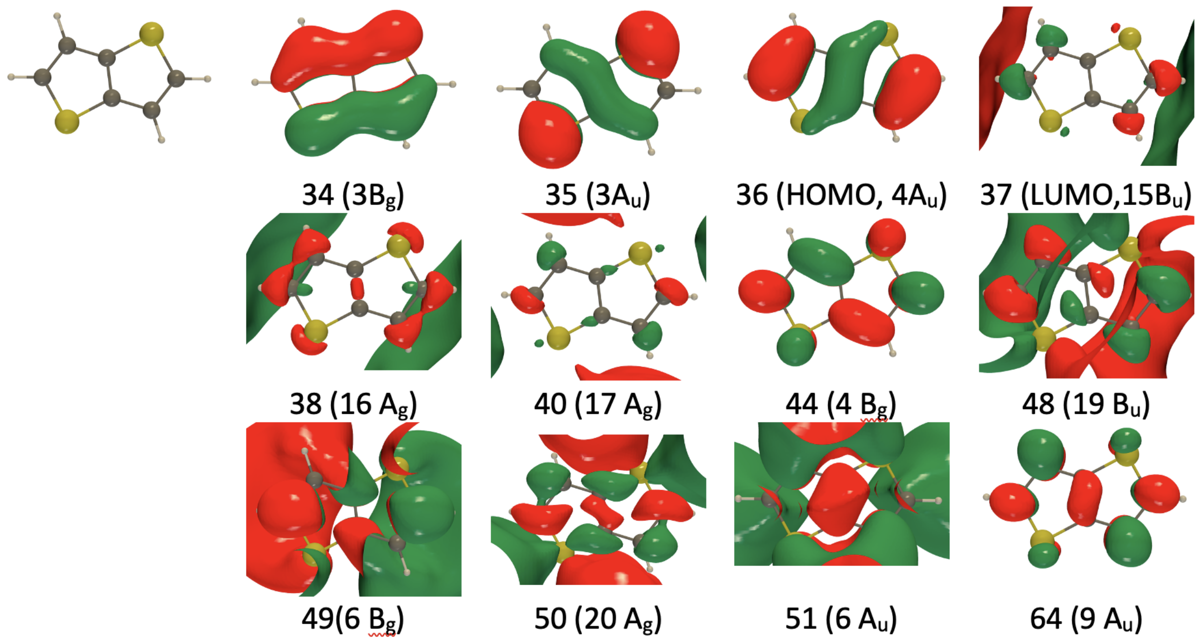

# S2 Cartesian coordinates

Below are the XYZ coordinates for all systems treated here (bohrs).

## S2.1 Azulene – CC3(FC)/cc-pVTZ

| | | | |
|---|---|---|---|
| C | 0.00000000 | 0.00000000 | -5.08442654 |
| C | 2.16799436 | 0.00000000 | -3.55850254 |
| C | -2.16799436 | 0.00000000 | -3.55850254 |
| C | 1.40560615 | 0.00000000 | -1.02382432 |
| C | -1.40560615 | 0.00000000 | -1.02382432 |
| C | 0.00000000 | 0.00000000 | 4.72891515 |
| C | 2.38587647 | 0.00000000 | 3.61219185 |
| C | -2.38587647 | 0.00000000 | 3.61219185 |
| C | 3.00158451 | 0.00000000 | 1.05184313 |
| C | -3.00158451 | 0.00000000 | 1.05184313 |
| H | 0.00000000 | 0.00000000 | -7.11850559 |
| H | 4.09656030 | 0.00000000 | -4.20278074 |
| H | -4.09656030 | 0.00000000 | -4.20278074 |
| H | 0.00000000 | 0.00000000 | 6.77201689 |
| H | 3.96514987 | 0.00000000 | 4.90481753 |
| H | -3.96514987 | 0.00000000 | 4.90481753 |
| H | 5.00047162 | 0.00000000 | 0.61482964 |
| H | -5.00047162 | 0.00000000 | 0.61482964 |

## S2.2 Benzooxadiazole – CC3(FC)/cc-pVTZ

| | | | |
|---|---|---|---|
| O | 0.00000000 | 0.00000000 | 4.23105351 |
| N | 0.00000000 | 2.15721782 | 2.80042430 |
| N | 0.00000000 | -2.15721782 | 2.80042430 |
| C | 0.00000000 | 1.34474119 | 0.44505130 |
| C | 0.00000000 | -1.34474119 | 0.44505130 |
| C | 0.00000000 | 2.73330026 | -1.85469062 |
| C | 0.00000000 | -2.73330026 | -1.85469062 |
| C | 0.00000000 | 1.35965956 | -4.03354365 |
| C | 0.00000000 | -1.35965956 | -4.03354365 |
| H | 0.00000000 | 4.76633138 | -1.84544064 |
| H | 0.00000000 | -4.76633138 | -1.84544064 |
| H | 0.00000000 | 2.32124878 | -5.82853313 |
| H | 0.00000000 | -2.32124878 | -5.82853313 |

## S2.3 Benzothiadiazole – CC3(FC)/cc-pVTZ

| | | | |
|---|---|---|---|
| S | 0.00000000 | 0.00000000 | 4.12782363 |
| N | 0.00000000 | 2.37994968 | 2.16794907 |
| N | 0.00000000 | -2.37994968 | 2.16794907 |
| C | 0.00000000 | 1.35464582 | -0.15090868 |
| C | 0.00000000 | -1.35464582 | -0.15090868 |
| C | 0.00000000 | 2.70608821 | -2.46599859 |
| C | 0.00000000 | -2.70608821 | -2.46599859 |
| C | 0.00000000 | 1.34964552 | -4.66429754 |
| C | 0.00000000 | -1.34964552 | -4.66429754 |
| H | 0.00000000 | 4.74051264 | -2.44976392 |
| H | 0.00000000 | -4.74051264 | -2.44976392 |
| H | 0.00000000 | 2.32640888 | -6.45161040 |
| H | 0.00000000 | -2.32640888 | -6.45161040 |

## S2.4 Diketopyrrolopyrrole – CC3(FC)/cc-pVTZ

| | | | |
|---|---|---|---|
| C | -0.78095706 | 1.10654573 | 0.00000000 |
| C | 0.78095706 | -1.10654573 | 0.00000000 |
| C | 0.75770683 | 3.16221974 | 0.00000000 |
| C | -0.75770683 | -3.16221974 | 0.00000000 |
| C | -3.42805036 | 0.33490251 | 0.00000000 |
| C | 3.42805036 | -0.33490251 | 0.00000000 |
| N | -3.23354900 | -2.34444494 | 0.00000000 |
| N | 3.23354900 | 2.34444494 | 0.00000000 |
| O | -5.40649570 | 1.49154645 | 0.00000000 |
| O | 5.40649570 | -1.49154645 | 0.00000000 |
| H | -4.76571395 | -3.46112039 | 0.00000000 |
| H | 4.76571395 | 3.46112039 | 0.00000000 |
| H | 0.30840723 | 5.14301221 | 0.00000000 |
| H | -0.30840723 | -5.14301221 | 0.00000000 |

## S2.5 Furofuran – CC3(FC)/cc-pVTZ

| | | | |
|---|---|---|---|
| C | 0.06548932 | 1.28240874 | 0.00000000 |
| C | -0.06548932 | -1.28240874 | 0.00000000 |
| C | -2.43794558 | 2.25427215 | 0.00000000 |
| C | 2.43794558 | -2.25427215 | 0.00000000 |
| C | -3.90023785 | 0.12403225 | 0.00000000 |
| C | 3.90023785 | -0.12403225 | 0.00000000 |
| O | 2.50066120 | 2.07485533 | 0.00000000 |
| O | -2.50066120 | -2.07485533 | 0.00000000 |
| H | -3.10620733 | 4.16541687 | 0.00000000 |
| H | 3.10620733 | -4.16541687 | 0.00000000 |
| H | -5.90761266 | -0.13384378 | 0.00000000 |
| H | 5.90761266 | 0.13384378 | 0.00000000 |

## S2.6 Phthalazine – CC3(FC)/cc-pVTZ

| | | | |
|---|---|---|---|
| C | 0.00000000 | 1.32459443 | -0.07132677 |
| C | 0.00000000 | -1.32459443 | -0.07132677 |
| C | 0.00000000 | 2.65486490 | -2.37693013 |
| C | 0.00000000 | -2.65486490 | -2.37693013 |
| C | 0.00000000 | 1.33510515 | -4.61541123 |
| C | 0.00000000 | -1.33510515 | -4.61541123 |
| C | 0.00000000 | 2.49806192 | 2.33813333 |
| C | 0.00000000 | -2.49806192 | 2.33813333 |
| N | 0.00000000 | 1.29575320 | 4.50170701 |
| N | 0.00000000 | -1.29575320 | 4.50170701 |
| H | 0.00000000 | 4.69409431 | -2.36246981 |
| H | 0.00000000 | -4.69409431 | -2.36246981 |
| H | 0.00000000 | 2.33538579 | -6.38945264 |
| H | 0.00000000 | -2.33538579 | -6.38945264 |
| H | 0.00000000 | 4.53863166 | 2.46976178 |
| H | 0.00000000 | -4.53863166 | 2.46976178 |

## S2.7 Pyrrolopyrrole – CC3(FC)/cc-pVTZ

| | | | |
|---|---|---|---|
| C | 0.01987029 | 1.31191436 | 0.00000000 |
| C | -0.01987029 | -1.31191436 | 0.00000000 |
| C | -2.50055820 | 2.23026347 | 0.00000000 |
| C | 2.50055820 | -2.23026347 | 0.00000000 |
| C | -3.99867844 | 0.09474099 | 0.00000000 |
| C | 3.99867844 | -0.09474099 | 0.00000000 |
| N | 2.50780926 | 2.04699311 | 0.00000000 |
| N | -2.50780926 | -2.04699311 | 0.00000000 |
| H | -3.17172573 | 4.14262242 | 0.00000000 |
| H | 3.17172573 | -4.14262242 | 0.00000000 |
| H | -6.02037705 | -0.05658473 | 0.00000000 |
| H | 6.02037705 | 0.05658473 | 0.00000000 |
| H | 3.16071224 | 3.82066088 | 0.00000000 |
| H | -3.16071224 | -3.82066088 | 0.00000000 |

## S2.8 Quinoxaline – CC3(FC)/cc-pVTZ

| | | | |
|---|---|---|---|
| C | 0.00000000 | 1.33833541 | 0.04624026 |
| C | 0.00000000 | -1.33833541 | 0.04624026 |
| C | 0.00000000 | 2.65319151 | -2.27752466 |
| C | 0.00000000 | -2.65319151 | -2.27752466 |
| C | 0.00000000 | 1.33717941 | -4.51073479 |
| C | 0.00000000 | -1.33717941 | -4.51073479 |
| C | 0.00000000 | 1.33936683 | 4.32768896 |
| C | 0.00000000 | -1.33936683 | 4.32768896 |
| N | 0.00000000 | 2.68409862 | 2.24219152 |
| N | 0.00000000 | -2.68409862 | 2.24219152 |
| H | 0.00000000 | 4.68915946 | -2.22328575 |
| H | 0.00000000 | -4.68915946 | -2.22328575 |
| H | 0.00000000 | 2.33972888 | -6.28367426 |
| H | 0.00000000 | -2.33972888 | -6.28367426 |
| H | 0.00000000 | 2.35369837 | 6.10018213 |
| H | 0.00000000 | -2.35369837 | 6.10018213 |

## S2.9 Tetrathiafulvalene – CC3(FC)/cc-pVTZ

| | | | |
|---|---|---|---|
| C | -1.27140171 | 0.00000000 | 0.00000000 |
| C | 1.27140171 | 0.00000000 | 0.00000000 |
| C | -5.98994256 | 1.26331812 | 0.00000000 |
| C | -5.98994256 | -1.26331812 | 0.00000000 |
| C | 5.98994256 | -1.26331812 | 0.00000000 |
| C | 5.98994256 | 1.26331812 | 0.00000000 |
| S | -3.07078317 | 2.82030107 | 0.00000000 |
| S | -3.07078317 | -2.82030107 | 0.00000000 |
| S | 3.07078317 | -2.82030107 | 0.00000000 |
| S | 3.07078317 | 2.82030107 | 0.00000000 |
| H | -7.66536437 | 2.41057807 | 0.00000000 |
| H | -7.66536437 | -2.41057807 | 0.00000000 |
| H | 7.66536437 | -2.41057807 | 0.00000000 |
| H | 7.66536437 | 2.41057807 | 0.00000000 |

## S2.10 Thienothiophene – CC3(FC)/cc-pVTZ

| | | | |
|---|---|---|---|
| C | 0.41618901 | 1.24091123 | 0.00000000 |
| C | -0.41618901 | -1.24091123 | 0.00000000 |
| C | -1.56128826 | 3.05660382 | 0.00000000 |
| C | 1.56128826 | -3.05660382 | 0.00000000 |
| C | -3.86882315 | 1.90421786 | 0.00000000 |
| C | 3.86882315 | -1.90421786 | 0.00000000 |
| S | 3.68518133 | 1.37661050 | 0.00000000 |
| S | -3.68518133 | -1.37661050 | 0.00000000 |
| H | -1.30761309 | 5.07161572 | 0.00000000 |
| H | 1.30761309 | -5.07161572 | 0.00000000 |
| H | -5.68944011 | 2.79705270 | 0.00000000 |
| H | 5.68944011 | -2.79705270 | 0.00000000 |

# S3 TBEs for all treated ESs

Table S11: TBE/*aug*-cc-pVTZ values (in eV) for all considered ESs alongside the CC3/*aug*-cc-pVTZ %$T_1$ (when available) as well as the protocol used to generate these TBEs. All values are obtained in the frozen-core approximation

| | State | %$T_1$ | TBE Value | Protocol |
|---|---|---|---|---|
| Azulene | $^1B_2$ (Val, $\pi \to \pi^\star$) | n.d. | 2.161 | CCSDT/6-31+G(d) + [CC3/AVTZ - CC3/6-31+G(d)] |
| | $^1A_1$ (CT, $\pi \to \pi^\star$) | n.d. | 3.849 | |
| | $^1B_2$ (CT, $\pi \to \pi^\star$) | n.d. | 4.510 | |
| | $^1A_2$ (Ryd.) | n.d. | 4.874 | |
| | $^1A_1$ (Val, $\pi \to \pi^\star$) | n.d. | 4.956 | |
| | $^1B_1$ (Ryd.) | n.d. | 5.302 | |
| | $^3B_2$ (Val, $\pi \to \pi^\star$) | n.d. | 2.180 | CC3/AVDZ + [CCSD/AVTZ - CCSD/AVDZ] |
| | $^3A_1$ (Val, $\pi \to \pi^\star$) | n.d. | 2.460 | |
| | $^3A_1$ (Val, $\pi \to \pi^\star$) | n.d. | 2.883 | |
| | $^3B_2$ (Val, $\pi \to \pi^\star$) | n.d. | 4.127 | |
| BOD | $^1B_2$ (Val, $\pi \to \pi^\star$) | 88.6 | 4.606 | CCSDT/AVDZ + [CC3/AVTZ - CC3/AVDZ] |
| | $^1A_1$ (Val, $\pi \to \pi^\star$) | 83.5 | 4.911 | |
| | $^1A_2$ (Val, $n \to \pi^\star$) | 86.9 | 5.312 | |
| | $^1B_1$ (Val, $n/\sigma \to \pi^\star$) | 85.6 | 5.849 | |
| | $^3B_2$ (Val, $\pi \to \pi^\star$) | 97.5 | 2.739 | CC3/AVTZ |
| | $^3A_1$ (Val, $\pi \to \pi^\star$) | 97.2 | 4.084 | |
| BTD | $^1B_2$ (CT, $\pi \to \pi^\star$) | 86.1 | 4.291 | CCSDT/AVDZ + [CC3/AVTZ - CC3/AVDZ] |
| | $^1A_1$ (Val, $\pi \to \pi^\star$) | 86.5 | 4.371 | |
| | $^1A_2$ (Val, $n \to \pi^\star$) | 87.7 | 4.806 | |
| | $^1B_1$ (Val, $n/\sigma \to \pi^\star$) | 86.1 | 5.422 | |
| | $^3B_2$ (Val, $\pi \to \pi^\star$) | 97.3 | 2.820 | CC3/AVTZ |
| | $^3A_1$ (Val, $\pi \to \pi^\star$) | 97.3 | 3.485 | |
| DPP | $^1B_u$ (Val, $\pi \to \pi^\star$) | 88.4 | 3.568 | CCSDT/6-31+G(d) + [CC3/AVTZ - CC3/6-31+G(d)] |
| | $^1A_u$ (Val, $n \to \pi^\star$) | 83.7 | 3.899 | |
| | $^1A_g$ (Val, $\pi \to \pi^\star$) | 87.0 | 3.960 | |
| | $^1B_g$ (Val, $n \to \pi^\star$) | 81.5 | 4.338 | |
| | $^3B_u$ (Val, $\pi \to \pi^\star$) | 97.4 | 1.927 | CC3/AVTZ |
| | $^3A_g$ (Val, $\pi \to \pi^\star$) | 97.3 | 3.743 | |
| | $^3A_u$ (Val, $n \to \pi^\star$) | 94.9 | 3.781 | |
| | $^3B_g$ (Val, $n \to \pi^\star$) | 94.5 | 4.226 | |
| FF | $^1A_u$ (Ryd) | 93.4 | 5.434 | CCSDT/AVDZ + [CC3/AVTZ - CC3/AVDZ] |
| | $^1B_u$ (Val, $\pi \to \pi^\star$) | 91.5 | 5.489 | |
| | $^1B_g$ (Ryd) | 93.4 | 5.865 | |
| | $^1B_g$ (Ryd) | 93.1 | 6.001 | |
| | $^1A_g$ (Val, $\pi \to \pi^\star$) | 82.6 | 6.027 | |
| | $^3B_u$ (Val, $\pi \to \pi^\star$) | 97.9 | 3.578 | CC3/AVTZ |
| | $^3A_g$ (Val, $\pi \to \pi^\star$) | 98.2 | 4.869 | |
| Phthalazine | $^1A_2$ (CT, $n \to \pi^\star$) | n.d. | 3.898 | CCSDT/6-31+G(d) + [CC3/AVTZ - CC3/6-31+G(d)] |
| | $^1B_1$ (CT, $n \to \pi^\star$) | n.d. | 4.302 | |
| | $^1A_1$ (Val, $\pi \to \pi^\star$) | n.d. | 4.451 | |
| | $^1B_2$ (Val, $\pi \to \pi^\star$) | n.d. | 5.188 | |
| | $^1B_1$ (CT, $n \to \pi^\star$) | n.d. | 5.548 | |
| | $^1A_2$ (Mixed) | n.d. | 5.842 | |
| | $^1A_2$ (CT, $n \to \pi^\star$) | n.d. | 5.876 | |
| | $^1A_1$ (Val, $\pi \to \pi^\star$) | n.d. | 6.109 | |
| | $^1A_2$ (Ryd) | n.d. | 6.444 | |
| | $^1B_2$ (Ryd) | n.d. | 6.263 | |
| | $^1A_1$ (Val, $\pi \to \pi^\star$) | n.d. | 6.408 | |

Continued on next page

| | State | $\%T_1$ | TBE Value | Protocol |
|---|---|---|---|---|
| | ${}^3B_2$ (Val, $\pi \rightarrow \pi^\star$) | 97.7 | 3.430 | CC3/AVTZ |
| | ${}^3A_2$ (CT, $n \rightarrow \pi^\star$) | 95.7 | 3.626 | |
| | ${}^3B_1$ (CT, $n \rightarrow \pi^\star$) | 96.1 | 3.711 | |
| | ${}^3A_1$ (Val, $\pi \rightarrow \pi^\star$) | 96.7 | 4.224 | |
| PP | ${}^1A_u$ (Ryd) | 92.8 | 4.536 | CCSDT/AVDZ + [CC3/AVTZ - CC3/AVDZ] |
| | ${}^1B_g$ (Ryd) | 92.5 | 4.739 | |
| | ${}^1A_u$ (Ryd) | 92.0 | 5.107 | |
| | ${}^1B_g$ (Ryd) | 93.1 | 5.133 | |
| | ${}^3B_u$ (Val, $\pi \rightarrow \pi^\star$) | 97.9 | 3.841 | CC3/AVTZ |
| | ${}^3A_u$ (Ryd) | 97.4 | 4.524 | |
| | ${}^3B_g$ (Ryd) | 97.3 | 4.733 | |
| Quinoxaline | ${}^1B_1$ (Val, $n \rightarrow \pi^\star$) | n.d. | 3.800 | CCSDT/6-31+G(d) + [CC3/AVTZ - CC3/6-31+G(d)] |
| | ${}^1A_1$ (Val, $\pi \rightarrow \pi^\star$) | n.d. | 4.248 | |
| | ${}^1B_2$ (CT, $\pi \rightarrow \pi^\star$) | n.d. | 4.641 | |
| | ${}^1A_2$ (Val, $n \rightarrow \pi^\star$) | n.d. | 5.100 | |
| | ${}^1A_2$ (Val, $n \rightarrow \pi^\star$) | n.d. | 5.388 | |
| | ${}^1A_1$ (CT, $\pi \rightarrow \pi^\star$) | n.d. | 5.665 | |
| | ${}^1B_1$ (CT, $n \rightarrow \pi^\star$) | n.d. | 6.205 | |
| | ${}^1B_2$ (Val, $\pi \rightarrow \pi^\star$) | n.d. | 6.299 | |
| | ${}^3B_2$ (Val, $\pi \rightarrow \pi^\star$) | 97.4 | 3.255 | CC3/AVTZ |
| | ${}^3B_1$ (Val, $n \rightarrow \pi^\star$) | 96.9 | 3.352 | |
| | ${}^3A_1$ (Val, $\pi \rightarrow \pi^\star$) | 96.9 | 3.875 | |
| TTF | ${}^1B_{3u}$ (Val, $\pi \rightarrow \sigma^\star$) | 90.1 | 2.800 | CCSDT/6-31+G(d) + [CC3/AVTZ - CC3/6-31+G(d)] |
| | ${}^1B_{2u}$ (Val, $\pi \rightarrow \pi^\star$) | 87.9 | 3.773 | |
| | ${}^1B_{1g}$ (Val, $\pi \rightarrow \sigma^\star$) | 90.5 | 3.987 | |
| | ${}^1B_{2g}$ (Val, $\pi \rightarrow \sigma^\star$) | 89.3 | 4.047 | |
| | ${}^1B_{3u}$ (Ryd.) | 92.8 | 4.114 | |
| | ${}^1B_{3g}$ (Val, $\pi \rightarrow \pi^\star$) | 86.2 | 4.243 | |
| | ${}^1B_{1u}$ (Val, $\pi \rightarrow \pi^\star$) | 90.6 | 4.525 | |
| | ${}^1B_{2g}$ (Ryd.) | 92.0 | 4.552 | |
| | ${}^3B_{3u}$ (Val, $\pi \rightarrow \sigma^\star$) | 96.7 | 2.652 | CC3/AVTZ |
| | ${}^3B_{1u}$ (Val, $\pi \rightarrow \pi^\star$) | 97.7 | 2.993 | |
| | ${}^3B_{2u}$ (Val,$\pi \rightarrow \pi^\star$) | 97.1 | 3.123 | |
| | ${}^3B_{3g}$ (Val, $\pi \rightarrow \pi^\star$) | 97.4 | 3.400 | |
| | ${}^3B_{1g}$ (Val, $\pi \rightarrow \sigma^\star$) | 96.8 | 3.803 | |
| | ${}^3B_{2g}$ (Val, $\pi \rightarrow \sigma^\star$) | 96.8 | 3.916 | |
| TT | ${}^1B_u$ (Val, $\pi \rightarrow \pi^\star$) | 87.5 | 4.965 | CCSDT/AVDZ + [CC3/AVTZ - CC3/AVDZ] |
| | ${}^1B_u$ (Val, $\pi \rightarrow \pi^\star$) | 90.6 | 5.243 | |
| | ${}^1B_g$ (Ryd) | 90.3 | 5.411 | |
| | ${}^1A_u$ (Ryd) | 91.6 | 5.509 | |
| | ${}^3B_u$ (Val, $\pi \rightarrow \pi^\star$) | 97.7 | 3.465 | CC3/AVTZ |
| | ${}^3B_u$ (Val, $\pi \rightarrow \pi^\star$) | 97.2 | 4.261 | |
| | ${}^3A_g$ (Val, $\pi \rightarrow \pi^\star$) | 97.9 | 4.580 | |

## S4 Raw benchmark data

Table S12: Transition energies determined with various models. All values are in eV and have been obtained with the *aug*-cc-pVTZ basis set applying the FC approximation. TM and QC stands for the Turbomole and Q-Chem packages that have different SOS parameters for spin-scaled ADC(2).

| | | TBE | CIS(D) | CC2 | EOM-MP2 | STEOM-CCSD | CCSD | CCSD(T)(a)* | CCSDR(3) | CCSDT-3 | CC3 | SOS-ADC(2) [TM] | SOS-CC2 [TM] | SCS-CC2 [TM] | SOS-ADC(2) [QC] | ADC(2) | ADC(3) | ADC(2.5) |
|---|---|---|---|---|---|---|---|---|---|---|---|---|---|---|---|---|---|---|
| Azulene | $^1B_2$ (Val, $\pi \to \pi^\star$) | 2.161 | 2.275 | 2.275 | 2.714 | | 2.278 | 2.250 | 2.254 | 2.200 | 2.169 | 2.194 | 2.221 | 2.243 | 1.973 | 2.228 | 1.986 | 2.107 |
| | $^1A_1$ (CT, $\pi \to \pi^\star$) | 3.849 | 4.098 | 3.893 | 4.349 | | 3.973 | 3.937 | 3.942 | 3.877 | 3.843 | 3.749 | 3.806 | 3.836 | 3.541 | 3.821 | 3.610 | 3.716 |
| | $^1B_2$ (CT, $\pi \to \pi^\star$) | 4.510 | 4.801 | 4.653 | 5.204 | | 4.780 | 4.657 | 4.641 | 4.579 | 4.491 | 4.591 | 4.607 | 4.619 | 4.364 | 4.633 | 4.416 | 4.525 |
| | $^1A_2$ (Ryd.) | 4.874 | 4.912 | 4.766 | 5.262 | | 4.903 | 4.897 | 4.905 | 4.888 | 4.855 | 4.965 | 4.925 | 4.874 | 4.838 | 4.790 | 4.702 | 4.746 |
| | $^1A_1$ (Val, $\pi \to \pi^\star$) | 4.956 | 4.984 | 4.820 | 5.498 | | 5.216 | 5.036 | 4.986 | 5.028 | 4.914 | 4.862 | 4.961 | 4.915 | 4.646 | 4.696 | 4.653 | 4.675 |
| | $^1B_1$ (Ryd.) | 5.302 | 5.284 | 5.175 | 5.668 | | 5.312 | 5.317 | 5.327 | 5.308 | 5.285 | 5.374 | 5.334 | 5.281 | 5.250 | 5.202 | 5.108 | 5.155 |
| | $^3B_2$ (Val, $\pi \to \pi^\star$) | 2.180 | 2.377 | 2.292 | 2.714 | | 2.199 | | | | | 2.331 | 2.379 | 2.351 | 2.139 | 2.227 | 1.842 | 2.035 |
| | $^3A_1$ (Val, $\pi \to \pi^\star$) | 2.460 | 2.859 | 2.672 | 4.349 | | 2.283 | | | | | 2.622 | 2.635 | 2.647 | 2.465 | 2.646 | 2.169 | 2.408 |
| | $^3A_1$ (Val, $\pi \to \pi^\star$) | 2.883 | 3.109 | 3.057 | 5.498 | | 2.924 | | | | | 2.991 | 3.012 | 3.028 | 2.806 | 3.024 | 2.546 | 2.785 |
| | $^3B_2$ (Val, $\pi \to \pi^\star$) | 4.127 | 4.424 | 4.347 | 5.204 | | 4.180 | | | | | 4.249 | 4.290 | 4.309 | 4.069 | 4.299 | 3.758 | 4.029 |
| BOD | $^1B_2$ (Val, $\pi \to \pi^\star$) | 4.606 | 4.906 | 4.687 | 5.209 | | 4.837 | 4.669 | 4.646 | 4.607 | 4.520 | 4.795 | 4.824 | 4.778 | 4.578 | 4.643 | 4.268 | 4.456 |
| | $^1A_1$ (Val, $\pi \to \pi^\star$) | 4.911 | 4.990 | 5.014 | 5.665 | | 5.221 | 5.078 | 5.070 | 4.999 | 4.906 | 5.066 | 5.092 | 5.061 | 4.799 | 4.919 | 4.328 | 4.624 |
| | $^1A_2$ (Val, $n \to \pi^\star$) | 5.312 | 5.755 | 5.264 | 6.030 | 5.212 | 5.576 | 5.443 | 5.442 | 5.380 | 5.284 | 5.719 | 5.728 | 5.580 | 5.463 | 5.220 | 5.158 | 5.189 |
| | $^1B_1$ (Val, $n/\sigma \to \pi^\star$) | 5.849 | 6.325 | 5.910 | 6.581 | | 6.148 | 5.996 | 5.996 | 5.930 | 5.833 | 6.312 | 6.303 | 6.178 | 6.057 | 5.883 | 5.603 | 5.743 |
| | $^3B_2$ (Val, $\pi \to \pi^\star$) | 2.739 | 3.193 | 3.008 | 3.142 | 2.365 | 2.635 | | | | 2.739 | 2.944 | 2.973 | 2.984 | 2.784 | 2.949 | 2.291 | 2.620 |
| | $^3A_1$ (Val, $\pi \to \pi^\star$) | 4.084 | 4.396 | 4.300 | 4.462 | 3.870 | 4.072 | | | | 4.084 | 4.142 | 4.218 | 4.248 | 3.957 | 4.129 | 3.696 | 3.913 |
| BTD | $^1B_2$ (CT, $\pi \to \pi^\star$) | 4.291 | 4.663 | 4.393 | 4.984 | 4.402 | 4.559 | 4.381 | 4.370 | 4.323 | 4.229 | 4.504 | 4.520 | 4.479 | 4.285 | 4.390 | 3.974 | 4.182 |
| | $^1A_1$ (Val, $\pi \to \pi^\star$) | 4.371 | 4.617 | 4.514 | 4.997 | | 4.540 | 4.470 | 4.467 | 4.411 | 4.359 | 4.454 | 4.442 | 4.465 | 4.223 | 4.513 | 4.141 | 4.327 |
| | $^1A_2$ (Val, $n \to \pi^\star$) | 4.806 | 5.151 | 4.720 | 6.130 | 4.681 | 5.019 | 4.922 | 4.925 | 4.868 | 4.795 | 5.095 | 5.071 | 4.958 | 4.851 | 4.733 | 4.770 | 4.752 |
| | $^1B_1$ (Val, $n/\sigma \to \pi^\star$) | 5.422 | 5.737 | 5.399 | 5.491 | | 5.694 | 5.551 | 5.553 | 5.503 | 5.417 | 5.796 | 5.756 | 5.642 | 5.552 | 5.435 | 5.343 | 5.389 |
| | $^3B_2$ (Val, $\pi \to \pi^\star$) | 2.820 | 3.262 | 3.055 | 3.261 | 2.484 | 2.739 | | | | 2.820 | 3.005 | 3.016 | 3.030 | 2.842 | 3.031 | 2.422 | 2.727 |
| | $^3A_1$ (Val, $\pi \to \pi^\star$) | 3.485 | 3.779 | 3.689 | 3.901 | 3.271 | 3.471 | | | | 3.485 | 3.615 | 3.637 | 3.655 | 3.440 | 3.645 | 3.106 | 3.376 |
| DPP | $^1B_u$ (Val, $\pi \to \pi^\star$) | 3.568 | 3.538 | 3.483 | 3.938 | | 3.738 | 3.576 | 3.567 | 3.598 | 3.535 | 3.612 | 3.740 | 3.653 | 3.376 | 3.313 | 3.418 | 3.366 |
| | $^1A_u$ (Val, $n \to \pi^\star$) | 3.899 | 4.030 | 3.812 | 4.431 | 3.939 | 4.282 | 4.061 | 4.048 | 3.998 | 3.863 | 4.202 | 4.360 | 4.187 | 3.933 | 3.653 | 4.243 | 3.948 |
| | $^1A_g$ (Val, $\pi \to \pi^\star$) | 3.960 | 4.117 | 3.937 | 4.506 | 3.696 | 4.209 | 4.029 | 4.030 | 4.013 | 3.910 | 4.219 | 4.214 | 4.122 | 3.974 | 3.937 | 3.912 | 3.925 |
| | $^1B_g$ (Val, $n \to \pi^\star$) | 4.338 | 4.549 | 4.329 | 4.862 | 4.415 | 4.745 | 4.540 | 4.524 | 4.450 | 4.309 | 4.615 | 4.808 | 4.661 | 4.347 | 4.124 | 4.693 | 4.409 |
| | $^3B_u$ (Val, $\pi \to \pi^\star$) | 1.927 | 2.211 | 2.014 | 2.237 | 1.667 | 1.879 | | | | 1.927 | 2.137 | 2.172 | 2.120 | 1.961 | 1.952 | 1.641 | 1.797 |
| | $^3A_g$ (Val, $\pi \to \pi^\star$) | 3.743 | 4.098 | 3.845 | 4.010 | 3.553 | 3.758 | | | | 3.743 | 3.981 | 4.023 | 3.972 | 3.811 | 3.787 | 3.486 | 3.637 |
| | $^3A_u$ (Val, $n \to \pi^\star$) | 3.781 | 3.982 | 3.690 | 4.267 | 3.839 | 4.109 | | | | 3.781 | 4.115 | 4.265 | 4.081 | 3.860 | 3.537 | 4.104 | 3.821 |
| | $^3B_g$ (Val, $n \to \pi^\star$) | 4.226 | 4.452 | 4.191 | 4.674 | 4.300 | 4.545 | | | | 4.226 | 4.512 | 4.694 | 4.536 | 4.261 | 3.992 | 4.544 | 4.268 |
| FF | $^1A_u$ (Ryd) | 5.434 | 5.527 | 5.416 | 5.778 | 5.489 | 5.522 | 5.460 | 5.466 | 5.449 | 5.430 | 5.660 | 5.595 | 5.535 | 5.456 | 5.483 | 5.285 | 5.384 |
| | $^1B_u$ (Val, $\pi \to \pi^\star$) | 5.489 | 5.740 | 5.542 | 5.907 | | 5.645 | 5.522 | 5.513 | 5.500 | 5.463 | 5.613 | 5.621 | 5.594 | 5.425 | 5.525 | 5.270 | 5.398 |
| | $^1B_g$ (Ryd) | 5.865 | 5.917 | 5.807 | 6.193 | 5.948 | 5.953 | 5.891 | 5.895 | 5.878 | 5.859 | 6.082 | 6.023 | 5.951 | 5.968 | 5.871 | 5.710 | 5.791 |
| | $^1B_g$ (Ryd) | 6.001 | 6.090 | 5.949 | 6.366 | 6.139 | 6.109 | 6.032 | 6.037 | 6.020 | 5.993 | 6.256 | 8.185 | 6.106 | 6.135 | 6.024 | 5.863 | 5.944 |
| | $^1A_g$ (Val, $\pi \to \pi^\star$) | 6.027 | 6.677 | 6.300 | 6.692 | | 6.433 | 6.265 | 6.209 | 6.146 | 6.040 | 6.428 | 6.419 | 6.380 | 6.216 | 6.319 | 5.652 | 5.986 |
| | $^3B_u$ (Val, $\pi \to \pi^\star$) | 3.578 | 3.921 | 3.793 | 3.858 | 3.408 | 3.516 | | | | 3.578 | 3.782 | 3.799 | 3.797 | 3.644 | 3.773 | 3.234 | 3.504 |
| | $^3A_g$ (Val, $\pi \to \pi^\star$) | 4.869 | 5.108 | 5.049 | 5.045 | 4.916 | 4.844 | | | | 4.869 | 4.951 | 4.968 | 4.996 | 4.826 | 5.009 | 4.569 | 4.789 |

Table S13: Transition energies determined with various models. See caption of Table S12 for more details.

| | | TBE | CIS(D) | CC2 | EOM-MP2 | STEOM-CCSD | CCSD | CCSD(T)(a)* | CCSDR(3) | CCSDT-3 | CC3 | SOS-ADC(2) [TM] | SOS-CC2 [TM] | SCS-CC2 [TM] | SOS-ADC(2) [QC] | ADC(2) | ADC(3) | ADC(2.5) |
|---|---|---|---|---|---|---|---|---|---|---|---|---|---|---|---|---|---|---|
| Phthalazine | $^1A_2$ (CT, $n \rightarrow \pi^\star$) | 3.898 | 4.280 | 3.756 | 4.465 | 3.880 | 4.247 | 4.027 | 4.020 | 4.011 | 3.872 | 4.274 | 4.276 | 4.111 | 4.017 | 3.759 | 4.193 | 3.976 |
| | $^1B_1$ (CT, $n \rightarrow \pi^\star$) | 4.302 | 4.717 | 4.185 | 4.909 | 4.253 | 4.608 | 4.435 | 4.427 | 4.401 | 4.283 | 4.670 | 4.671 | 4.514 | 4.420 | 4.184 | 4.477 | 4.331 |
| | $^1A_1$ (Val, $\pi \rightarrow \pi^\star$) | 4.451 | 4.655 | 4.600 | 5.072 | 4.259 | 4.642 | 4.574 | 4.578 | 4.519 | 4.473 | 4.530 | 4.526 | 4.550 | 4.291 | 4.613 | 4.362 | 4.488 |
| | $^1B_2$ (Val, $\pi \rightarrow \pi^\star$) | 5.188 | 5.522 | 5.110 | 5.656 | 5.230 | 5.368 | 5.246 | 5.240 | 5.214 | 5.146 | 5.246 | 5.279 | 5.232 | 5.041 | 5.103 | 5.042 | 5.073 |
| | $^1B_1$ (CT, $n \rightarrow \pi^\star$) | 5.548 | 5.451 | 5.349 | 6.134 | 5.565 | 5.908 | 5.656 | 5.658 | 5.660 | 5.520 | 5.956 | 5.952 | 5.784 | 5.701 | 5.444 | 5.865 | 5.655 |
| | $^1A_2$ (Mixed) | 5.842 | | 5.494 | 6.787 | | 6.541 | 6.067 | 6.052 | 6.042 | 5.744 | 6.626 | 6.461 | 6.119 | 6.211 | 5.533 | 6.641 | 6.087 |
| | $^1A_2$ (CT, $n \rightarrow \pi^\star$) | 5.876 | 5.827 | 5.811 | 6.529 | 5.884 | 6.224 | 6.012 | 6.013 | 5.985 | 5.870 | 6.322 | 6.314 | 6.157 | 6.073 | 5.817 | 6.055 | 5.936 |
| | $^1A_1$ (Val, $\pi \rightarrow \pi^\star$) | 6.109 | 6.440 | 6.286 | 6.807 | 6.115 | 6.422 | 6.279 | 6.282 | 6.231 | 6.148 | 6.253 | 6.294 | 6.260 | 6.010 | | 5.855 | 2.928 |
| | $^1A_2$ (Ryd) | 6.444 | 6.483 | 6.379 | 6.812 | 6.558 | 6.517 | 6.464 | 6.459 | 6.461 | 6.430 | 6.625 | 6.577 | 6.511 | 6.503 | 6.432 | 6.285 | 6.359 |
| | $^1B_2$ (Ryd) | 6.263 | | 5.697 | 6.777 | 6.569 | 6.546 | 6.373 | 6.367 | 6.403 | 6.234 | 6.615 | | 6.253 | 6.412 | 5.781 | | |
| | $^1A_1$ (Val, $\pi \rightarrow \pi^\star$) | 6.408 | 6.442 | 6.368 | 6.977 | | 6.650 | 6.504 | 6.429 | 6.456 | 6.364 | 6.541 | 6.553 | 6.486 | 6.329 | | 6.297 | 3.149 |
| | $^3B_2$ (Val, $\pi \rightarrow \pi^\star$) | 3.430 | 3.850 | 3.587 | 3.763 | 3.015 | 3.319 | | | | 3.430 | 3.497 | 3.652 | 3.632 | 3.498 | 3.589 | 3.171 | 3.380 |
| | $^3A_2$ (CT, $n \rightarrow \pi^\star$) | 3.626 | 4.089 | 3.514 | 4.095 | 3.622 | 3.891 | | | | 3.626 | 3.778 | 4.015 | 3.854 | 3.779 | 3.506 | 3.832 | 3.669 |
| | $^3B_1$ (CT, $n \rightarrow \pi^\star$) | 3.711 | 4.105 | 3.682 | 4.168 | 3.507 | 3.899 | | | | 3.711 | 3.898 | 4.120 | 3.977 | 3.899 | 3.676 | 3.740 | 3.708 |
| | $^3A_1$ (Val, $\pi \rightarrow \pi^\star$) | 4.224 | 4.660 | 4.426 | 4.710 | 4.122 | 4.315 | | | | 4.224 | 4.197 | 4.394 | 4.407 | 4.198 | 4.413 | 3.941 | 4.177 |
| PP | $^1A_u$ (Ryd) | 4.536 | 4.596 | 4.485 | 4.911 | 4.689 | 4.653 | 4.580 | 4.587 | 4.565 | 4.545 | 4.747 | 4.691 | 4.623 | 4.628 | 4.547 | 4.454 | 4.501 |
| | $^1B_g$ (Ryd) | 4.739 | 4.794 | 4.676 | 5.129 | 4.945 | 4.842 | 4.788 | 4.794 | 4.772 | 4.746 | 5.577 | 4.921 | 4.839 | 4.855 | 4.742 | 4.664 | 4.703 |
| | $^1A_u$ (Ryd) | 5.107 | 5.194 | 4.947 | 5.461 | 5.238 | 5.191 | 5.162 | 5.169 | 5.166 | 5.133 | 5.254 | 5.208 | 5.120 | 5.107 | 4.976 | 5.164 | 5.070 |
| | $^1B_g$ (Ryd) | 5.133 | 5.118 | 5.040 | 5.467 | 5.263 | 5.201 | 5.171 | 5.178 | 5.157 | 5.145 | 5.805 | 5.234 | 5.169 | 5.167 | 5.092 | 5.045 | 5.069 |
| | $^3B_u$ (Val, $\pi \rightarrow \pi^\star$) | 3.841 | 4.164 | 4.016 | 4.122 | | 3.782 | | | | 3.841 | 4.006 | 4.017 | 4.017 | 3.865 | 4.007 | 3.562 | 3.785 |
| | $^3A_u$ (Ryd) | 4.524 | 4.592 | 4.469 | 5.110 | 4.589 | 4.596 | | | | 4.524 | 4.739 | 4.684 | 4.613 | 4.622 | 4.530 | 4.428 | 4.479 |
| | $^3B_g$ (Ryd) | 4.733 | 4.791 | 4.663 | 4.880 | 4.826 | 4.823 | | | | 4.733 | 4.973 | 4.915 | 4.832 | 4.851 | 4.730 | 4.648 | 4.689 |
| Quinoxaline | $^1B_1$ (Val, $n \rightarrow \pi^\star$) | 3.800 | 4.025 | 3.732 | 4.331 | 3.726 | 4.016 | 3.889 | 3.888 | 3.865 | 3.790 | 4.158 | 4.128 | 4.001 | 3.925 | 3.765 | 3.830 | 3.798 |
| | $^1A_1$ (Val, $\pi \rightarrow \pi^\star$) | 4.248 | 4.449 | 4.387 | 4.872 | 4.062 | 4.428 | 4.359 | 4.362 | 4.308 | 4.263 | 4.311 | 4.303 | 4.331 | 4.074 | 4.402 | 4.118 | 4.260 |
| | $^1B_2$ (CT, $\pi \rightarrow \pi^\star$) | 4.641 | 5.070 | 4.565 | 5.246 | 4.721 | 4.906 | 4.721 | 4.714 | 4.690 | 4.586 | 4.768 | 4.791 | 4.719 | 4.542 | 4.565 | 4.542 | 4.554 |
| | $^1A_2$ (Val, $n \rightarrow \pi^\star$) | 5.100 | 5.449 | 4.997 | 5.646 | 5.127 | 5.383 | 5.206 | 5.201 | 5.195 | 5.087 | 5.441 | 5.419 | 5.287 | 5.196 | 5.021 | 5.237 | 5.129 |
| | $^1A_2$ (Val, $n \rightarrow \pi^\star$) | 5.388 | 5.723 | 5.469 | 6.107 | 5.453 | 5.811 | 5.581 | 5.575 | 5.525 | 5.390 | 5.899 | 5.880 | 5.729 | 5.652 | 5.486 | 5.563 | 5.525 |
| | $^1A_1$ (CT, $\pi \rightarrow \pi^\star$) | 5.665 | 5.840 | 5.739 | 6.278 | | 5.912 | 5.774 | 5.769 | 5.751 | 5.674 | 5.744 | 5.739 | 5.745 | 5.516 | 5.734 | 5.517 | 5.626 |
| | $^1B_1$ (CT, $n \rightarrow \pi^\star$) | 6.205 | | 6.020 | 7.001 | | 6.726 | 6.370 | 6.360 | 6.355 | 6.140 | 6.842 | 6.780 | 6.524 | 6.586 | 6.097 | 6.677 | 6.387 |
| | $^1B_2$ (Val, $\pi \rightarrow \pi^\star$) | 6.299 | 6.811 | 6.342 | 6.799 | | 6.487 | 6.372 | 6.363 | 6.339 | 6.277 | 6.340 | 6.361 | 6.351 | 6.139 | 6.323 | 6.136 | 6.230 |
| | $^3B_2$ (Val, $\pi \rightarrow \pi^\star$) | 3.255 | 3.708 | 3.411 | 3.636 | 2.871 | 3.173 | | | | 3.255 | 3.468 | 3.474 | 3.455 | 3.309 | 3.414 | 2.995 | 3.205 |
| | $^3B_1$ (Val, $n \rightarrow \pi^\star$) | 3.352 | 3.612 | 3.312 | 3.784 | 3.196 | 3.494 | | | | 3.352 | 3.733 | 3.714 | 3.582 | 3.524 | 3.331 | 3.320 | 3.326 |
| | $^3A_1$ (Val, $\pi \rightarrow \pi^\star$) | 3.875 | 4.195 | 4.030 | 4.345 | 3.756 | 3.923 | | | | 3.875 | 4.043 | 4.047 | 4.042 | 3.858 | 4.032 | 3.547 | 3.790 |

Table S14: Transition energies determined with various models. See caption of Table S12 for more details.

| | | TBE | CIS(D) | CC2 | EOM-MP2 | STEOM-CCSD | CCSD | CCSD(T)(a)* | CCSDR(3) | CCSDT-3 | CC3 | SOS-ADC(2) [TM] | SOS-CC2 [TM] | SCS-CC2 [TM] | SOS-ADC(2) [QC] | ADC(2) | ADC(3) | ADC(2.5) |
|---|---|---|---|---|---|---|---|---|---|---|---|---|---|---|---|---|---|---|
| TTF | $^1B_{3u}$ (Val, $\pi \to \sigma^\star$) | 2.800 | 2.845 | 2.700 | 3.128 | 2.800 | 3.019 | 2.863 | 2.863 | 2.865 | 2.787 | 3.267 | 3.228 | 3.055 | 3.087 | 2.765 | 2.784 | 2.775 |
| | $^1B_{2u}$ (Val, $\pi \to \pi^\star$) | 3.773 | 3.858 | 3.568 | 4.197 | 3.910 | 4.088 | 3.856 | 3.851 | 3.855 | 3.742 | 4.216 | 4.195 | 3.988 | 4.017 | 3.623 | 3.894 | 3.759 |
| | $^1B_{1g}$ (Val, $\pi \to \sigma^\star$) | 3.987 | 4.160 | 3.887 | 4.329 | 4.100 | 4.194 | 4.026 | 4.057 | 4.054 | 3.979 | 4.447 | 4.399 | 4.234 | 4.281 | 3.970 | 3.994 | 3.982 |
| | $^1B_{2g}$ (Val, $\pi \to \sigma^\star$) | 4.047 | 4.156 | 3.981 | 4.348 | 4.033 | 4.238 | 4.134 | 4.125 | 4.113 | 4.048 | 4.455 | 4.411 | 4.273 | 4.296 | 4.054 | 3.996 | 4.025 |
| | $^1B_{3u}$ (Ryd.) | 4.114 | 4.050 | 3.905 | 4.390 | 4.222 | 4.224 | 4.148 | 4.155 | 4.153 | 4.113 | 4.469 | 4.386 | 4.226 | 4.347 | 4.008 | 4.099 | 4.054 |
| | $^1B_{3g}$ (Val, $\pi \to \pi^\star$) | 4.243 | 4.503 | 4.076 | 4.668 | | 4.584 | 4.351 | 4.342 | 4.339 | 4.218 | 4.659 | 4.658 | 4.469 | 4.456 | 4.106 | 4.360 | 4.233 |
| | $^1B_{1u}$ (Val, $\pi \to \pi^\star$) | 4.525 | 4.468 | 4.338 | 4.773 | 4.480 | 4.681 | 4.541 | 4.537 | 4.571 | 4.514 | 4.649 | 4.695 | 4.575 | 4.459 | 4.270 | 4.535 | 4.403 |
| | $^1B_{2g}$ (Ryd.) | 4.552 | 4.540 | 4.354 | 4.828 | 4.601 | 4.683 | 4.586 | 4.598 | 4.600 | 4.551 | 4.898 | 4.835 | 4.676 | 4.764 | 4.434 | 4.542 | 4.488 |
| | $^3B_{3u}$ (Val, $\pi \to \sigma^\star$) | 2.652 | 2.784 | 2.546 | 2.941 | 2.629 | 2.840 | | | | 2.652 | 3.126 | 3.093 | 2.913 | 2.958 | 2.603 | 2.629 | 2.616 |
| | $^3B_{1u}$ (Val, $\pi \to \pi^\star$) | 2.993 | 3.239 | 2.975 | 3.188 | | 2.961 | | | | 2.993 | 3.154 | 3.166 | 3.105 | 3.003 | 2.948 | 2.820 | 2.884 |
| | $^3B_{2u}$ (Val,$\pi \to \pi^\star$) | 3.123 | 3.585 | 3.048 | 3.342 | 3.003 | 3.211 | | | | 3.123 | 3.418 | 3.411 | 3.304 | 3.269 | 3.073 | 3.050 | 3.062 |
| | $^3B_{3g}$ (Val, $\pi \to \pi^\star$) | 3.400 | 3.791 | 3.374 | 3.564 | 3.242 | 3.438 | | | | 3.400 | 3.629 | 3.633 | 3.558 | 3.487 | 3.372 | 3.275 | 3.324 |
| | $^3B_{1g}$ (Val, $\pi \to \sigma^\star$) | 3.803 | 4.029 | 3.709 | 4.087 | 3.863 | 3.972 | | | | 3.803 | 4.247 | 4.211 | 4.049 | 4.091 | 3.777 | 3.788 | 3.783 |
| | $^3B_{2g}$ (Val, $\pi \to \sigma^\star$) | 3.916 | 4.074 | 3.850 | 4.141 | 3.852 | 4.056 | | | | 3.916 | 4.306 | 4.279 | 4.140 | 4.155 | 3.900 | 3.851 | 3.876 |
| TT | $^1B_u$ (Val, $\pi \to \pi^\star$) | 4.965 | 4.998 | 4.981 | 5.348 | | 5.165 | 5.037 | 5.034 | 5.032 | 4.964 | 5.112 | 5.138 | 5.086 | 4.899 | 4.948 | 4.972 | 4.960 |
| | $^1B_u$ (Val, $\pi \to \pi^\star$) | 5.243 | 5.481 | 5.285 | 5.701 | | 5.395 | 5.284 | 5.279 | 5.261 | 5.224 | 5.340 | 5.346 | 5.327 | 5.151 | 5.276 | 5.068 | 5.172 |
| | $^1B_g$ (Ryd) | 5.411 | 5.660 | 5.386 | 5.719 | 5.482 | 5.600 | 5.517 | 5.494 | 5.476 | 5.412 | 5.761 | 5.730 | 5.628 | 5.610 | 5.466 | 5.375 | 5.421 |
| | $^1A_u$ (Ryd) | 5.509 | 5.616 | 5.445 | 5.843 | 5.592 | 5.647 | 5.586 | 5.579 | 5.560 | 5.518 | 5.810 | 5.734 | 5.639 | 5.682 | 5.530 | 5.453 | 5.492 |
| | $^3B_u$ (Val, $\pi \to \pi^\star$) | 3.465 | 3.820 | 3.643 | 3.776 | 3.149 | 3.391 | | | | 3.465 | 3.631 | 3.635 | 3.629 | 3.489 | 3.636 | 3.153 | 3.395 |
| | $^3B_u$ (Val, $\pi \to \pi^\star$) | 4.261 | 4.522 | 4.363 | 4.520 | 4.111 | 4.312 | | | | 4.261 | 4.419 | 4.445 | 4.421 | 4.253 | 4.324 | 4.100 | 4.212 |
| | $^3A_g$ (Val, $\pi \to \pi^\star$) | 4.580 | 4.846 | 4.717 | 4.780 | 4.442 | 4.555 | | | | 4.580 | 4.655 | 4.661 | 4.683 | 4.525 | 4.693 | 4.330 | 4.512 |
